# Supplementary material for: Semantic Segmentation in Satellite Hyperspectral Imagery by Deep Learning
Source: arXiv:2310.16210 source file (2024-10-25)
Supplement: Supplementary file 1 [file APPENDICES_FOR_EXTENDED_THESIS.tex]

\clearpage
\appendix

\section{NOT PART OF THIS PAPER Extended Methodology + State of the art review for the PhD thesis}
\jon{This note is written on 14th October 2023. I have now written the results and the methodology needs to be further compressed since as Radu mentions it has much verbrose including many basic details of Machine Learning and Deep Learning Models. So, what I am doing is to move the methodology as it is now to this appendix section and I will compress and modify/restructure/rewrite the methodology. This previous extended methodology can be used to provide further lower-level and basic details for the extended version of the thesis. NOTE: The section is commented out to avoid messing with the label commands with the rest of the text}

\section{NOT PART OF THIS PAPER . Extended State-of-the-art Review for the PhD thesis}

\jon{Commented out the extended state of the art to avoid that citations appear in the manuscript.}
